# Supplementary material for: FPT Algorithms for Conflict-free Coloring of Graphs and Chromatic Terrain Guarding
Source: arXiv:1905.01822 source file (2019-05-06)
Supplement: Supplementary file 1 [file appendix1.tex]

\begin{lemma}~\label{jointnodelemma1}
Recurrence for the join node for \textsc{k - Conflict free Coloring} is correct.
\end{lemma}
\begin{proof}

We prove the correctness of the recurrence for the case where $f(v) = B$ and $(f_1(v), f_2(v)) \in \{(B,C), (C,B) \}$ (proof of the other cases can be obtained using similar arguments). We show that $d[t, c, \gamma, f] = d[t_1, c, \gamma, f_1] \wedge d[t_2, c, \gamma, f_2]$ if for every $v \in X_t$, $c(v)=c_1(v)=c_2(v)$ and $\gamma(v)=\gamma_1(v)=\gamma_2(v)$, and $f(v) = B$ and $(f_1(v), f_2(v)) \in \{(B,C), (C,B) \}$. Without loss of generality, assume,  $(f_1(v), f_2(v)) = (B, C)$.

We analyze both the cases, the first case where $d[t_1, c, \gamma, f_1] = d[t_2, c, \gamma, f_2] = true$, and the second case where one of $(d[t_1, c, \gamma, f_1]$ and $d[t_2, c, \gamma, f_2])$ is true and the other is false.

\noindent \textbf{Case 1 - $d[t_1, c, \gamma, f_1] = d[t_2, c, \gamma, f_2] = true$}:
Let ${\sf col}: V(G_{t_1}) \rightarrow \{c_0,c_1,\ldots,c_k\}$ be a $(t_1, c , \gamma ,f_1)$-good coloring, and let ${\sf col}: V(G_{t_2}) \rightarrow \{c_0,c_1,\ldots,c_k\}$ be a $(t_2, c , \gamma ,f_2)$-good coloring. We can note that there is exactly one vertex $u_1 \in N_{G_{t_1}}[v]$, such that ${\sf col}(u_1) = \gamma(v)$ since $f_1(v) = B$. Since the vertex $u_1$ can conflict-free color the vertex $v$ through an introduce edge node of $v u_1$, the vertex $u_1$ must have been subsequently forgotten in $G_{t_1}$. Similarly, since $f_2(v) = C$, we can also note that for every $u \in N_{G_{t_1}}[v]$, we have ${\sf col}(u) \neq \gamma(v)$. Now, notice that in the coloring  $(t, c , \gamma ,f)$, $u_1$ is the unique vertex in $N_{G_t}[v]$ where ${\sf col}(u_1) = \gamma(v)$. For every other vertex $u \neq u_1$ in $N_{G_t}[v]$, we know that ${\sf col}(u_1) \neq \gamma(v)$. Hence, we can conclude that ${\sf col} : V(G_t) \rightarrow \{c_0,c_1,\ldots,c_k\}$ is a $(t, c, \gamma ,f)$-good coloring, which implies $d[t, c, \gamma, f] = true$.

\noindent \textbf{Case 2 - $(d[t_1, c, \gamma, f_1], d[t_2, c, \gamma, f_2]) \in \{(false,true), (true,false)\}$}:
Assume $d[t_1, c, \gamma, f_1] = true$ and $d[t_2, c, \gamma, f_2] = false$. This essentially states that the coloring $c$ is invalid for $G_{t_2}$, and hence will be invalid for $G_t$ as well. Hence, $d[t, c, \gamma, f] = false$.

The two cases together prove that $d[t, c, \gamma, f] = d[t_1, c, \gamma, f_1] \wedge d[t_2, c, \gamma, f_2]$ for the case considered.

\end{proof}

\begin{lemma}~\label{join_node_scfc}
Recurrence for the join node for \textsc{k-Strong Conflict-Free Coloring} is correct.
\end{lemma}
\begin{proof}

We prove the correctness of the recurrence for the case where $f(v) = W$ and $(f_1(v), f_2(v)) \in \{(W,R), (R,W) \}$. We show that $d[t, c, \Gamma, f] = d[t_1, c_1, \Gamma_1, f_1] \wedge d[t_2, c_2, \Gamma_2, f_2]$ if for every $v \in X_t$, $c(v)=c_1(v)=c_2(v)$, the values of $\Gamma(v), \Gamma_1(v), \Gamma_2(v)$ are \textit{consistent}, i.e., as described in the recurrence, and $f(v) = W$ and $(f_1(v), f_2(v)) \in \{(W,R), (R,W) \}$. Without loss of generality, assume,  $(f_1(v), f_2(v)) = (W, R)$.

We analyze both the cases, the first case where $d[t_1, c_1, \Gamma_1, f_1] = d[t_2, c, \Gamma_2, f_2] = true$, and the second case where one of $(d[t_1, c, \Gamma, f_1]$ and $d[t_2, c, \Gamma, f_2])$ is true and the other is false.

\noindent \textbf{Case 1 - $d[t_1, c, \gamma, f_1] = d[t_2, c, \gamma, f_2] = true$}:Let ${\sf col}: V(G_{t_1}) \rightarrow \{c_0,c_1,\ldots,c_k\}$ be a $(t_1, f_1, c_1, \Gamma_1)$-good coloring, and let ${\sf col}: V(G_{t_2}) \rightarrow \{c_0,c_1,\ldots,c_k\}$ be a $(t_2, f_2, c_2, \Gamma_2)$-good coloring. Since $f_1(v) = W$, we can note that for every $i \in [k]$, where $\Gamma_1(v)[i] = 1$, there is exactly one vertex $u_1 \in N_{G_{t_1}}[v]$, such that ${\sf col}(u_1) = \Gamma(v)[i]$ since $f_1(v) = W$. Similarly, since $f_2(v) = R$, we can also note that for every $i \in [k]$, $\Gamma_2(v)[i] \in \{(0, \hat{1})\}$, i.e., there is no vertex $u \in N_{G_{t_2}}[v]$ such that we have ${\sf col}(u) = c_i$, for $c_i \neq c_0$ Now, for tuples $(t_1, f_1, c_1, \Gamma_1)$ and $(t_2, f_2, c_2, \Gamma_2)$ to be $(t, f, c, \Gamma)$-consistent, the values of $\Gamma(v)$ must be \textit{consistent} with $\Gamma_1(v)$ and $\Gamma_1(v)$. Assume for some $j$, $(\Gamma_1(v)[j], \Gamma_2(v)[j]) = (1, \hat{1})$. For the tuples to be consistent, we require that $\Gamma(v)[j] = 1$. In tuple $(t, f, c, \Gamma)$, we can note that for color $j$, there is exactly one vertex $u_1 \in N_{G_t}[v]$ such that ${\sf col}(u_1) = \Gamma(v)[j]$, and for every vertex $u \neq u_1$ in $N_{G_t}[v]$, ${\sf col}(u) \neq c_j$. Likewise, assume for some $j'$, $(\Gamma_1(v)[j'], \Gamma_2(v)[j']) = (0, 0)$. This implies that $\Gamma(v)[j'] = 0$. Again, in tuple $(t, f, c, \Gamma)$, we can note that for color $j'$, there is no neighbor $u \in N_{G_t}[v]$ such that ${\sf col}(v) = c_{j'}$. Hence, we can conclude that ${\sf col} : V(G_t) \rightarrow \{c_0,c_1,\ldots,c_k\}$ is a $(t, f, c, \gamma)$-good coloring, which implies $d[t, c, \gamma, f] = true$.

\noindent \textbf{Case 2 - $(d[t_1, c, \gamma, f_1], d[t_2, c, \gamma, f_2]) \in \{(false,true), (true,false)\}$}:
Assume $d[t_1, c, \gamma, f_1] = true$ and $d[t_2, c, \gamma, f_2] = false$. The argument here is similar to that of conflict-free coloring and proves that $d[t, c, \gamma, f] = false$.

The two cases together prove that $d[t, c, \gamma, f] = d[t_1, c, \gamma, f_1] \wedge d[t_2, c, \gamma, f_2]$ for the case considered.

\end{proof}
