# Supplementary material for: FPT Algorithms for Conflict-free Coloring of Graphs and Chromatic Terrain Guarding
Source: arXiv:1905.01822 source file (2019-05-06)
Supplement: Supplementary file 2 [file appendix.tex]

\begin{lemma}~\label{jointnodelemma1}
Recurrence for the join node for \textsc{k - Conflict free Coloring} is correct.
\end{lemma}
\begin{proof}

Consider the join node $X_t$. Let $d[t,c,\gamma,f]=true$. We prove that there exists $[t_1,c_1,\gamma_1,f_1]$ and $[t_2,c_2,\gamma_2,f_2]$, such that the pair is  $(t,c,\gamma,f)$-consistent and $d[t_1,c_1,\gamma_1,f_1] =true$ and $d[t_2,c_2,\gamma_2,f_2] = true$.  For every vertex $v$, we assign $c_1(v)=c_2(v)=c(v)$ and $\gamma_1(v)=\gamma_2(v)=\gamma(v)$. We define $f_1$ and $f_2$ for the vertex $v$ as follows: 

\noindent \emph{Case 1: $f(v)=W$} :   Let $\gamma(v)=c_i$. Since $d[t_1,c,\gamma,f]=true$, $G_t$ admits a conflict free coloring where $v$ is conflict free dominated by a vertex, say $u$, with color $c_i$. Without loss of generality, let $u$ be a neighbor of $v$ in $G_{t_1}$. Assign $f_1(v)=W$ and $f_2(v)=G$. Note that $u\in V_{t_1}\setminus X_t$. Therefore $v$ is conflict free dominated in $G_{t_1}$ by the same coloring restricted to $V_t$ and $d[t_1,c_1,\gamma_1,f_1]=true$. We will show that $d[t_2,c_2,\gamma_2,f_2]=true$. For contradiction, assume not. Therefore, in any coloring of $G_{t_2}$, $v$ is already conflict free dominated by a vertex with color $c_i$. This implies that in the conflict free coloring of $G_t$ corresponding to $[c,\gamma,f]$, $v$ has a neighbor with color $c_i$, other than $u$. This contradicts that $d[t,c,\gamma,f]=true$. Similarly we can prove that $d[t,c,\gamma,f]=true$ when $d[t_1,c_1,\gamma_1,f_1]=d[t_2,c_2,\gamma_2,f_2]=true$.
\vspace{5pt}
\noindent\emph{Case 2: $f(v)=B$} : When $c(v)=\gamma(v)$ , $v$ is conflict free dominated by itself in $G_t$ if and only if it is also conflict free dominated by itself in $G_{t_1}$ and $G_{t_2}$ and the recurrence holds. Assume $c(v) \ne \gamma(v)$. Let $d[t, c, \gamma, f] = true$. Then there exists a conflict free coloring of $V_t$ where $v$ is conflict free colored by a vertex $u \ne v$ in $G_t$. Without loss of generality, assume $u \in V_{t_1}$. Assign $f_1(v)=B $ and $f_2(v)=C$. We can show that $d[t_1, c, \gamma, f_1]=d[t_2, c, \gamma, f_2]=true$ by similar arguments as in Case 1.
\vspace{5pt}
\noindent\emph{Case 3: $f(v)=C$ or $f(v)=W$} : $f(v)=C$ and $d[t, c, \gamma, f] = true$ implies there exists a conflict free coloring of $G_t$ where $v$ is colored but is not conflict free dominated by any neighbors. Since $G_{t_1}$ and $G_{t_2}$ are subgraphs of $G_{t}$ , $d[t_1, c, \gamma, f] = d[t_2, c, \gamma, f] = true$. Similarly we can prove the reverse direction. The case $f(v)=G$ is similar.
\end{proof}
